# Supplementary material for: Relation of the Relations: A New Paradigm of the Relation Extraction Problem
Source: arXiv:2006.03719 source file (2020-10-12)
Supplement: Supplementary file 1 [file additional_secs.tex]

\subsection{The Tradeoff between precision and recall}
\begin{table*}[!ht]
  
  \centering
  \resizebox{\textwidth}{!}{
    \begin{tabular}{l|ccc|ccc|ccc|ccc|ccc}
    \toprule
     & \multicolumn{3}{c|}{\textbf{BC\_dev}} & \multicolumn{3}{c|}{\textbf{BC\_test}} & \multicolumn{3}{c|}{\textbf{CTS}} & \multicolumn{3}{c|}{\textbf{WL}} & \multicolumn{3}{c}{\textbf{Overall}} \\
     & \textbf{P} & \textbf{R} & \textbf{Micro} & \textbf{P} & \textbf{R} & \textbf{Micro} & \textbf{P} & \textbf{R} & \textbf{Micro} & \textbf{P} & \textbf{R} & \textbf{Micro} & \textbf{P} & \textbf{R} & \textbf{Micro} \\
     \hline
     
    \textbf{$\text{\modelname{}}$}  & 76.76 & 64.25 & 69.8& 71.64 & \textbf{62.08} & 67.17& 63.52 & \textbf{60.25} & 59.5& 60.89 & \textbf{54.77} & 58.4 & 65.35
& \textbf{59.03}
& 61.69\\
    \textbf{$\text{\modelname{}}_\text{local}$}   & 77.01 & 61.69 & 68.44& \textbf{77.52} & 61.94 & 68.89& \textbf{71.95} &  57.93 & 59.87& 65.51 & 54.61 & 60.6 & \textbf{71.66}
& 58.16
& 63.12\\
    \textbf{$\text{\modelname{}}_\text{non-local}$} & 79.57 & \textbf{65.15} & \textbf{70.97}& 72.64 & 61.78 & 67.88& 69.14 & 52.84 & 58.55& 63.17 & 52.96 & 58.52 & 68.32
& 55.86
& 61.65\\
    \textbf{$\text{\modelname{}}_\text{glocal}$} & \textbf{80.30} & 62.98 & 70.36& 77.03 & 61.88 & \textbf{69.82}& 70.20 & 59.64 & \textbf{61.17}& \textbf{65.94} & 54.48 & \textbf{61.7} & 71.06

&58.67& \textbf{64.23}\\
    \bottomrule
    \end{tabular}
  }
  \caption{Precision and Recall on ACE05} \label{tab:addlabel}
\end{table*}

\begin{table}[htbp]
  \centering
    \begin{tabular}{lccc}
    \toprule
    \textbf{Model}    & \textbf{P} & \textbf{R} & \textbf{Micro} \\
    \midrule
    \multicolumn{4}{c}{\textbf{\emph{Non-ensemble models}}} \\
           \textbf{$\text{\modelname{}}$}  & 32.05 & \textbf{49.37} & 37.9 \\
           \textbf{$\text{\modelname{}}_\text{local}$}   & 39.31 & 45.3  & 39.24 \\
           \textbf{$\text{\modelname{}}_\text{non-local}$}  & 39.08 & 47.68 & 39.63 \\
           \textbf{$\text{\modelname{}}_\text{glocal}$}  & \textbf{44.24} & 46.86 & \textbf{39.74} \\
    \midrule
    \multicolumn{4}{c}{\textbf{\emph{Ensemble models}}} \\
           \textbf{E-$\text{\modelname{}}$}  & 40.77 & \textbf{54.03} & 42.39 \\
           \textbf{E-$\text{\modelname{}}_\text{local}$}    & 51.03 & 51.98 & 43.12 \\
           \textbf{E-$\text{\modelname{}}_\text{non-local}$}  & 52.31 & 51.39 & \textbf{43.98} \\
           \textbf{E-$\text{\modelname{}}_\text{glocal}$}  & \textbf{56.48} & 47.44 & 43.35 \\
    \bottomrule
    \end{tabular}%  
    \caption{Results on SemEval 2018 Task 7.2}

  \label{tab:res_semeval}%
\end{table}%

\subsection{Which model captures which feature well?}

2. example
\subsection{Ablation Study on ACE05}

\subsection{Two-Stage Training}
We study the performance of each stage in the two-stage learning on ACE05 validation set in Table~\ref{tab:ablation}. The first stage is binary classification to distinguish whether two entities have ``no-relation'' or a valid relation. In this stage, the glocal model which combines both the local learner and non-local supervisor performs the best, scoring +2.55 F1 scores higher than the base model.

We observe that in both datasets, there are a dominant number of negative labels. The experiments show that the difficulty is more in identifying whether there exists a relation, than in classifying the specific relation. So it is also worth exploring a two-stage learning strategy for local and non-local correlations. Following \cite{DBLP:journals/corr/abs-1909-11898}, in the first stage, we train an extraction model on identifying binary relations (where the ``no-relation'' label is treated as negative, and all other relations are positive). In the second stage, a classification model, which is trained to classify the different positive relations, will be applied on the samples which the extraction model in Stage 1 labels as positive. We denote the combination of a local extracting model and local classification model as \textbf{$\text{\modelname{}}_{\text{ex:local},  \text{cl:local}}$}, and the combination of a glocal extracting model and local classification model as \textbf{$\text{\modelname{}}_{\text{ex:glocal}, \text{cl:local}}$}.
